# Supplementary material for: A Poisson-Gamma Dynamic Factor Model with Time-Varying Transition Dynamics
Source: arXiv:2402.16297 source file (2024-05-23)
Supplement: Supplementary file 1 [file supplementary.tex]

\normalsize
\appendix
%\glsresetall
%\section{Notations}
%11111

\section{MCMC Inference}
\noindent\textbf{Notation.}
When expressing the full conditionals for Gibbs sampling, we use the shorthand ``--'' to denote all other variables.
We use ``$\boldsymbol{\cdot}$'' as an index summation shorthand, e.g., $x_{\boldsymbol{\cdot} j} = \sum_i x_{ij}$. 

In this section, we present a fully-conjugate and efficient Gibbs sampler for the proposed NS-PGDS. The sampling algorithms depend on several key technical results, which we will repeatedly exploit, thus we list them below.

\noindent\textbf{Negative Binomial Distribution}  
Let $y \sim \mathrm{Pois} \left( c \lambda \right)$, and $\lambda \sim \mathrm{Gam} \left( a, b\right)$. If we marginalize over $\lambda$, then $y \sim \mathrm{NB} \left( a, \frac{c}{b+c} \right)$ is a negative-binomial distributed random variable. We can further parameterize it as $y \sim \mathrm{NB} \left( a, g \left( \zeta \right) \right)$, where $g\left( z \right) = 1 - \mathrm{exp} \left( -z \right)$ and $\zeta = \mathrm{ln} \left( 1 + \frac{c}{b} \right)$.

\noindent\textbf{Lemma~1.}
If $y \sim \mathrm{NB} \left( a, g \left( \zeta \right) \right)$ and $l \sim \mathrm{CRT} \left( y, a\right)$, where $\mathrm{CRT} \left( \cdot \right)$ represents Chinese restaurant table distribution~\cite{YWT2006hier}, then the joint distribution of $y$ and $l$ can be equivalently distributed as $y \sim \mathrm{SumLog} \left( l, g \left( \zeta \right) \right)$ and $l \sim \mathrm{Pois} \left( a \zeta \right)$~\cite{zhou2015negative}, i.e.
    $$
        \mathrm{NB} \left(y; a, g \left( \zeta \right) \right) \mathrm{CRT} \left(l; y, a\right) =  \mathrm{SumLog} \left(y; l, g \left( \zeta \right) \right) \mathrm{Pois} \left(l; a \zeta \right),
    $$
    where $\mathrm{SumLog} \left(l, g \left( \zeta \right) \right) = \sum_{i=1}^l x_i$ and $x_i \sim \mathrm{Log} \left( 
    g \left( \zeta \right) \right)$ are independently and identically logarithmic distributed random variables~\cite{johnson2005univariate}.

\noindent\textbf{Lemma~2.}
Suppose $\mathbf{n} = \left( n_1, \cdots, n_K\right)$ and
    $
        \mathbf{n} \mid n \sim \mathrm{DirMult} \left( n, r_1, \cdots, r_K \right),
    $
    where $\mathrm{DirMult} \left( \cdot \right)$ refers to Dirichlet-multimonial distribution. We sample augmented variable $q \mid n \sim \mathrm{Beta}\left( n, r_{\cdot}\right)$,
    where $r_{\cdot} = \sum_{k=1}^K r_k$. According to~\cite{zhou2018nonparametric}, conditioning on $q$, we have $n_k \sim \mathrm{NB} \left( r_k, q\right)$.
    
\noindent\textbf{Lemma~3.}
If $y_{\cdot} = \sum_{s=1}^{S} y_s$, and $y_s \stackrel{\text{i.i.d}}{\sim} \mathrm{Pois} \left( \lambda_s \right), s=1,\cdots,S$. Then $y_{\cdot} \sim \mathrm{Pois} \left( \sum_{s=1}^{S} \lambda_s \right)$ and $\left( y_1, \cdots, y_S\right) \sim \mathrm{Mult} \left( y_{\cdot}, \left( \frac{\lambda_1}{\sum_{s=1}^{S} \lambda_s}, \cdots, \frac{\lambda_S}{\sum_{s=1}^{S} \lambda_s} \right) \right)$, where $\mathrm{Mult} \left( \cdot \right)$ represents multinomial distribution~\cite{kingman1992poisson}.
\\
\noindent\textbf{Sampling $y_{vk}^{(t)}$:} Use the relationship between Poisson and multinomial distributions as described by Lemma 3, given observed counts and latent parameters, we sample
\begin{equation}
\label{y_vk}
    \left( \left( y_{vk}^{(t)} \right)_{k=1}^K \mid - \right) \sim \mathrm{Mult} \left( y_v^{(t)}, \left( \frac{\phi_{vk} \theta_k^{(t)}}{\sum_{k=1}^K \phi_{vk} \theta_k^{(t)}} \right)_{k=1}^K \right).
\end{equation}
Then the distribution of $y_{vk}^{(t)}$ is $y_{vk}^{(t)} \sim \mathrm{Pois} \left( \delta^{(t)} \phi_{vk} \theta_k^{(t)} \right)$.
%\begin{equation}
%    y_{vk}^{(t)} \sim \mathrm{Pois} \left( \delta^{(t)} \phi_{vk} \theta_k^{(t)} \right).
%\end{equation}
\\
\noindent\textbf{Sampling $\bm{\phi_k}$:} Via Dirichlet-multinomial conjugacy, the posterior of $\boldsymbol{\phi_k}$ is
\begin{equation}
\label{phi_k}
    \left( \boldsymbol{\phi_k} \mid -\right) \sim \mathrm{Dir} \left( \epsilon_0 + \sum_{t=1}^T y_{1k}^{(t)}, \cdots, \epsilon_0 + \sum_{t=1}^T y_{Vk}^{(t)}\right).
\end{equation}
\\
\noindent\textbf{Marginalizing over $\theta_k^{(t)}$:} Note that $y_v^{(t)} = y_{v \cdot}^{(t)} = \sum_{k=1}^K y_{vk}^{(t)}$ and $y_{vk}^{(t)} \sim \mathrm{Pois} \left( \delta^{(t)} \phi_{vk} \theta_k^{(t)} \right)$. Then we define $y_{\cdot k}^{(t)} = \sum_{v=1}^V y_{vk}^{(t)}$. Because $\sum_{v=1}^V \phi_{vk} = 1$, we obtain $y_{\cdot k}^{(t)} \sim \mathrm{Pois} \left( \delta^{(t)} \theta_k^{(t)} \right)$. 

We start by marginalizing over $\theta_k^{(T)}$, using the definition of negative binomial distribution, we obtain
\begin{equation}
    y_{\cdot k}^{(T)} \sim \mathrm{NB} \left( \tau_0 \sum_{k_2=1}^K \pi_{kk_2}^{i\left( T-1 \right)}\theta_{k_2}^{\left( T-1 \right)} , g \left( \zeta^{(T)} \right)\right), \nonumber
\end{equation}
where $\zeta^{(T)} = \mathrm{ln} \left( 1 + \frac{\delta^{(T)}}{\tau_0} \right)$. Next, we further marginalize over $\theta_k^{(T-1)}$. To this end, we first sample auxiliary variables 
\begin{equation}
l_k^{(T)} \sim \mathrm{CRT} \left( y_{\cdot k}^{(T)}, \tau_0 \sum_{k_2=1}^K \pi_{kk_2}^{i\left( T-1 \right)} \theta_{k_2}^{(T-1)} \right). \nonumber
\end{equation}
By Lemma 1, the joint distribution of $y_{\cdot k}^{(T)}$ and $l_k^{(T)}$ can be expressed as 
\begin{equation}
    y_{\cdot k}^{(T)} \sim \mathrm{SumLog} \left( l_k^{(T)}, g \left( \zeta^{(T)} \right) \right) \; \mathrm{and} \; l_k^{(T)}  \sim \mathrm{Pois}\left( \zeta^{(T)} \tau_0 \sum_{k_2=1}^K \pi_{kk_2}^{i\left( T-1 \right)} \theta_{k_2}^{(T-1)} \right). \nonumber
\end{equation}
Via Lemma 3, we re-express the auxiliary variables as
\begin{equation}
    l_k^{(T)}  = l_{k \cdot}^{(T)} = \sum_{k_2=1}^K l_{kk_2}^{(T)}, \; \mathrm{and \; obtain} \; l_{kk_2}^{(T)} \sim \mathrm{Pois} \left( \zeta^{(T)} \tau_0 \pi_{kk_2}^{i\left( T-1\right)} \theta_{k_2}^{(T-1)} \right). \nonumber
\end{equation}
Then we define $l_{\cdot k}^{(T)} = \sum_{k_1=1}^K l_{k_1k}^{(T)}$. Leveraging Lemma 3 and $\sum_{k_1=1}^K \pi_{k_1k}^{i\left( T-1 \right)} = 1$, we obtain
\begin{align}
\label{l_tk}
    l_{\cdot k}^{(T)} \sim \mathrm{Pois} \left( \zeta^{(T)} \tau_0 \theta_k^{(T-1)} \right) \; \mathrm{and} \; \left( l_{1k}^{(T)}, \cdots, l_{Kk}^{(T)} \right) \sim \nonumber \mathrm{Mult} \left( l_{\cdot k}^{(T)}, \left( \pi_{1k}^{i\left( T-1 \right)} , \cdots, \pi_{Kk}^{i\left( T-1 \right)} \right) \right).
\end{align}
Next, note that $y_{\cdot k}^{(T-1)} \sim \mathrm{Pois} \left( \delta^{(T-1)} \theta_k^{(T-1)} \right)$, if we introduce $m_k^{(T-1)} = y_{\cdot k}^{(T-1)} + l_{\cdot k}^{(T)}$, then we have
\begin{equation}
    m_k^{(T-1)} \sim \mathrm{Pois} \left( \theta_k^{(T-1)} \left( \delta^{(T-1)} + \zeta^{(T)} \tau_0 \right) \right). \nonumber
\end{equation}
Because the prior of $\theta_k^{(T-1)}$ is gamma distributed, by the definition of negative binomial distribution, we can again marginalize over $\theta_k ^{(T-1)}$ to obtain
\begin{equation}
    m_k^{(T-1)} \sim \mathrm{NB} \left( \tau_0 \sum_{k_2=1}^K \pi_{kk_2}^{i\left( T-2\right)} \theta_{k_2}^{(T-2)} , g \left( \zeta^{(T-1)} \right)\right), \nonumber
\end{equation}
where $\zeta^{(T-1)} = \mathrm{ln} \left( 1 + \frac{\delta^{(T-1)}}{\tau_0} + \zeta^{(T)} \right)$. Then we introduce auxiliary variables 
\begin{equation}
l_{k}^{(T-1)} \sim \mathrm{CRT} \left( m_k^{(T-1)},  \tau_0 \sum_{k_2=1}^K \pi_{kk_2}^{i\left( T-2\right)} \theta_{k_2}^{(T-2)} \right). \nonumber
\end{equation}
And similar to the case for $t=T$, we can obtain
\begin{align}
     l_{\cdot k}^{(T-1)} \sim \mathrm{Pois} \left( \zeta^{(T-1)} \tau_0 \theta_k^{(T-2)} \right) \; \mathrm{and} \; m_k^{(T-2)} \sim \mathrm{NB} \left( \tau_0 \sum_{k_2=1}^K \pi_{kk_2}^{i\left( T-3\right)} \theta_{k_2}^{(T-3)} , g \left( \zeta^{(T-2)} \right)\right). \nonumber
\end{align}
Thus we have marginalized over $\theta_k^{(T-2)}$. Note that we can repeat this marginalization process recursively until $t=1$ with $\zeta^{(t)} = \mathrm{ln} \left( 1 + \frac{\delta^{(t)}}{\tau_0} + \zeta^{(t+1)} \right)$ and $m_k^{(T)} = y_{\cdot k}^{(T)}$ to maginalize over all the $\theta_k^{(t)}$.
\\
\noindent \textbf{Sampling $\theta_k^{(t)}$ :} Via the above marginalization process, to sample from the posterior of $\theta_k^{(t)}$, we first sample the auxiliary variables. Set $l_{\cdot k}^{(T+1)} = 0$ and $\zeta^{(T+1)} = 0$, sampling backwards from $t = T, \cdots, 2$,
\begin{align}
    \left( l_{k\cdot}^{(t)} \mid - \right) & \sim \mathrm{CRT} \left( y_{\cdot k}^{(t)} + l_{\cdot k}^{(t+1)}, \tau_0 \sum_{k_2=1}^K \pi_{kk_2}^{i\left( t-1 \right)} \theta_{k_2}^{(t-1)} \right), \label{l_k} \\
    \left( l_{k1}^{(t)}, \cdots, l_{kK}^{(t)} \mid - \right) & \sim \mathrm{Mult} \left( l_{k\cdot}^{(t)}, \left(\frac{\pi_{k1}^{i\left( t-1 \right)} \theta_1^{(t-1)}}{\sum_{k_2=1}^{K} \pi_{kk_2}^{i\left( t-1 \right)} \theta_{k_2}^{(t-1)} }, \cdots, \frac{\pi_{kK}^{i\left( t-1 \right)} \theta_K^{(t-1)}}{\sum_{k_2=1}^{K} \pi_{kk_2}^{i\left( t-1 \right)} \theta_{k_2}^{(t-1)} } \right) \right). \label{l_kk}
\end{align}
And via Lemma 3, we obtain
\begin{equation}
    \left( l_{1k}^{(t)}, \cdots, l_{Kk}^{(t)} \right) \sim \mathrm{Mult}\left(l_{\cdot k}^{(t)}, \pi_{1k}^{i\left( t-1 \right)},\cdots,\pi_{Kk}^{i\left( t-1 \right)}\right) \label{l_kk_mult}
\end{equation}
We compute $\zeta^{(t)}$ recursively via
%\begin{align}
%    l_{\cdot k}^{(t+1)} &= \sum_{k_1=1}^K l_{k_1k}^{(t)}, \\
%    \zeta^{(t)} & = \mathrm{ln} \left( 1 + \frac{\delta^{(t)}}{\tau_0} + \zeta^{(t+1)} \right).
%\end{align}
\begin{equation}
    \zeta^{(t)} = \mathrm{ln} \left( 1 + \frac{\delta^{(t)}}{\tau_0} + \zeta^{(t+1)} \right).
\end{equation}
After sampling the auxiliary variables, then for $t=1, \cdots, T$, by Poisson-gamma conjugacy, we obtain
\begin{align}
    \left( \theta_k^{(1)} \mid - \right) & \sim \mathrm{Gam} \left( y_{\cdot k}^{(1)} + l_{\cdot k}^{(2)} + \tau_0 \nu_k,  \tau_0 + \delta^{(1)} + \zeta^{(2)} \tau_0 \right), \label{theta_1}\\
    \left( \theta_k^{(t)} \mid - \right) & \sim \mathrm{Gam} \left( y_{\cdot k}^{(t)} + l_{\cdot k}^{(t+1)} + \tau_0 \sum_{k_2=1}^K \pi_{kk_2}^{i\left( t-1\right)} \theta_{k_2}^{(t-1)}, \tau_0 + \delta^{(t)} + \zeta^{(t+1)} \tau_0 \right).\label{theta_t}
\end{align}
\\
\noindent\textbf{Sampling $\bm{\Pi}^{(i)}$ :} We define $M$ as the length of each interval, and $I$ as the number of intervals. For $i=I$, by Eq.(\ref{l_kk_mult}), $\left( l_{1k}^{(I)}, \cdots, l_{Kk}^{(I)}\right)$ is multinomial distributed. Thus by multinomial-Dirichlet conjugacy, we obtain
\begin{equation}
\label{pi_I}
    \left( \boldsymbol{\pi}_k^{(I)} \mid -\right) \sim \mathrm{Dir}\left( \alpha_{1k}^{(I)} + l_{1k}^{(I)}, \cdots, \alpha_{Kk}^{(I)} + l_{Kk}^{(I)} \right).
\end{equation}
Where $l_{k_1k}^{(I)}$ indicates the summation of $l_{k_1k}^{(t)}$ over $I$-th interval, i.e. $l_{k_1k}^{(I)} = \sum_{t=(I-1)M+1}^T l_{k_1k}^{(t)}$. 

\noindent \textbf{Inference for Dirichlet-Dirichlet Markov chains.} For Dirichlet-Dirichlet Markov chains, $\alpha_{k_1k}^{\left(i \right)} = \eta K \pi_{k_1k}^{\left(i-1\right)}$. By Eq.(\ref{l_kk_mult}), $\left( l_{1k}^{(i)}, \cdots, l_{Kk}^{(i)}\right)$ is multinomial distributed. If we marginalize $\left( \pi_{1k}^{(i)}, \cdots, \pi_{Kk}^{(i)} \right)$, $\left( l_{1k}^{(i)}, \cdots, l_{Kk}^{(i)}\right)$ will be Dirichlet-multinomial distributed. Thus by Lemma 2, for $i=I$, we first sample the auxiliary variables as
\begin{align}
    \left( q_k^{(I)} \mid -\right) \sim \mathrm{Beta} \left( l_{\cdot k}^{(I)}, \eta K\right) \; \mathrm{and} \; \left(h_{k_1k}^{(I)} \mid - \right) \sim \mathrm{CRT} \left( l_{k_1k}^{(I)}, \eta K \pi_{k_1k}^{\left(I-1\right)}\right). \label{q_h_I}
\end{align}
Similarly, by Eq.(\ref{h_mult}), $\left( h_{1k}^{(i)},\cdots, h_{Kk}^{(i)} \right)$ is also Dirichlet-multinomial distributed. Thus for $i=I-1,\cdots,2$, we sample the auxiliary variables as
\begin{align}
    \left( q_k^{(i)} \mid -\right) \sim \mathrm{Beta} \left( l_{\cdot k}^{(i)} + h_{\cdot k}^{(i+1)}, \eta K\right) \; \mathrm{and} \; \left(h_{k_1k}^{(i)} \mid - \right) \sim \mathrm{CRT} \left( l_{k_1k}^{(i)} + h_{k_1 k}^{(i+1)}, \eta K \pi_{k_1k}^{\left(i-1\right)}\right). \label{q_h_i}
\end{align}
Where $l_{k_1k}^{(i)} = \sum_{\left( i-1 \right)M+1}^{iM}l_{k_1k}^{(t)}$ refers to the summation of $l_{k_1k}^{(t)}$ over $i$-th interval. Via Lemma 2, conditioning on $q_k^{(i)}$, we have
\begin{equation}
    \left( l_{k_1k}^{(i)} + h_{k_1 k}^{(i+1)}\right) \sim \mathrm{NB} \left( \eta K \pi_{k_1k}^{\left(i-1\right)}, q_k^{(i)} \right). \nonumber
\end{equation}
Then via Lemma 1, we obtain
\begin{equation}
\label{h_iK}
    h_{k_1k}^{(i)} \sim \mathrm{Pois} \left( -\eta K \pi_{k_1k}^{\left(i-1\right)} \mathrm{ln} \left( 1 - q_k^{(i)} \right) \right).
\end{equation}
Note that by Eq.(\ref{h_iK}), $h_{k_1k}^{(i)}$ is Poisson distributed and by Lemma 3, we obtain
\begin{equation}
\label{h_mult}
    \left( h_{1k}^{(i)}, \cdots, h_{Kk}^{(i)} \right) \sim \mathrm{Mult} \left(h_{\cdot k}^{(i)}, \left( \pi_{1k}^{(i-1)}, \cdots, \pi_{Kk}^{(i-1)} \right)\right).
\end{equation}
In addition, note that
\begin{equation}
\label{l_mult}
\begin{aligned}
    \left( l_{1k}^{(i-1)}, \cdots, l_{Kk}^{(i-1)}\right) \sim \mathrm{Mult}\left(l_{\cdot k}^{(i-1)}, \left( \pi_{1k}^{(i-1)}, \cdots, \pi_{Kk}^{(i-1)} \right)\right), \nonumber
\end{aligned}
\end{equation}
Via Dirichlet-multinomial conjugacy, for $i=I-1, \cdots, 2$, we obtain
\begin{equation}
\label{pi_i}
    \left( \boldsymbol{\pi}_k^{(i)} \mid -\right) \sim \mathrm{Dir} \left(  \eta K \pi_{1k}^{(i-1)} + l_{1k}^{(i)} + h_{1k}^{\left(i+ 1\right)}, \cdots,  \eta K \pi_{Kk}^{(i-1)} + l_{Kk}^{(i)} + h_{Kk}^{\left(i+1 \right)}\right).
\end{equation}
Specifically, for $i=1$, we have
\begin{equation}
\label{pi_1}
    \left( \boldsymbol{\pi}_k^{(1)} \mid - \right) \sim \mathrm{Dir} \left( \nu_1 \nu_k + l_{1k}^{(1)} + h_{1k}^{(2)}, \cdots, \xi \nu_k + l_{kk}^{(1)} + h_{kk}^{(2)}, \cdots,\nu_K \nu_k + l_{Kk}^{(1)} + h_{Kk}^{(2)} \right).
\end{equation}
For sampling $\eta$, note that $\left( h_{k_1k}^{(i)} \mid - \right) \sim \mathrm{Pois} \left( -\eta K \pi_{k_1k}^{(i-1)} \mathrm{ln} \left( 1 - q_k^{(i)} \right) \right)$, $i=I, \cdots, 2$. Given the prior $\eta \sim \mathrm{Gam} \left( e_0, f_0 \right)$, via Poisson-gamma conjugacy, we obtain
\begin{equation}
\label{eta}
    \left( \eta \mid - \right) \sim \mathrm{Gam} \left( e_0 + \sum_{i=2}^I \sum_{k_1=1}^K \sum_{k_2=1}^K h_{k_1k_2}^{(i)}, f_0 - K \sum_{i=2}^I \sum_{k=1}^K \mathrm{ln} \left( 1 - q_k^{(i)} \right) \right).
\end{equation}

\noindent \textbf{Inference for Dirichlet-Gamma-Dirichlet Markov chains.} For Dirichlet-Gamma-Dirichlet Markov chains
\begin{equation}
    \alpha_{k_1k}^{(i)} \sim \mathrm{Gam} \left( \gamma_k^{(i-1)} \sum_{k2=1}^K \psi^{(i-1)}_{kk_1k_2}\pi_{k_2k}^{(i-1)}, c_k^{(i)} \right). \nonumber
\end{equation}
By Eq.(\ref{l_kk_mult}), $\left( l_{1k}^{(i)}, \cdots, l_{Kk}^{(i)}\right)$ is multinomial distributed. If we marginalize $\left( \pi_{1k}^{(i)}, \cdots, \pi_{Kk}^{(i)} \right)$, $\left( l_{1k}^{(i)}, \cdots, l_{Kk}^{(i)}\right)$ will be Dirichlet-multinomial distributed. Thus by Lemma 2, for $i=I$, we first sample the auxiliary variables as
\begin{align}
    \left( q_k^{(I)} \mid -\right) \sim \mathrm{Beta} \left( l_{\cdot k}^{(I)}, \alpha_{\cdot k}^{(I)}\right) \; \mathrm{and} \; \left(h_{k_1k}^{(I)} \mid - \right) \sim \mathrm{CRT} \left( l_{k_1k}^{(I)}, \alpha_{k_1k}^{(I)}\right). \label{q_h_I_gam}
\end{align}
Similarly, by Eq.(\ref{g_mult_gam}), $\left( g_{\cdot 1k}^{(i)},\cdots, g_{\cdot Kk}^{(i)} \right)$ is also Dirichlet-multinomial distributed. Thus for $i=I-1,\cdots,2$, we sample the auxiliary variables as
\begin{align}
    \left( q_k^{(i)} \mid -\right) \sim \mathrm{Beta} \left( l_{\cdot k}^{(i)} + g_{\cdot k}^{(i+1)}, \alpha_{\cdot k}^{(i)}\right) \; \mathrm{and} \; \left(h_{k_1k}^{(i)} \mid - \right) \sim \mathrm{CRT} \left( l_{k_1k}^{(i)} + g_{\cdot k_1 k}^{(i+1)}, \alpha_{k_1k}^{(i)}\right). \label{q_h_i_gam}
\end{align}
Via Lemma 2, conditioning on $q_k^{(i)}$, we have
\begin{equation}
    \left( l_{k_1k}^{(i)} + g_{\cdot k_1 k}^{(i+1)}\right) \sim \mathrm{NB} \left( \alpha_{k_1k}^{(i)}, q_k^{(i)} \right). \nonumber
\end{equation}
Then via Lemma 1, we obtain
\begin{equation}
\label{H_iK_gam}
    h_{k_1k}^{(i)} \sim \mathrm{Pois} \left( -\alpha_{k_1k}^{(i)} \mathrm{ln} \left( 1 - q_k^{(i)} \right) \right). \nonumber
\end{equation}
Thus via Poisson-gamma conjugacy, we obtain
\begin{equation}
\label{alpha_gam}
    \left( \alpha_{k_1k}^{(i)} \mid - \right) \sim \mathrm{Gam} \left( \gamma_k^{(i-1)} \sum_{k2=1}^K \psi^{(i-1)}_{kk_1k_2}\pi_{k_2k}^{(i-1)} + h_{k_1k}^{(i)}, c_k^{(i)}-\mathrm{ln}\left( 1-q_k^{(i)}\right)\right).
\end{equation}
Marginalizing over $\alpha_{k_1k}^{(i)}$, and via the definition of negative binomial distribution, we have
\begin{equation}
    h_{k_1k}^{(i)} \sim \mathrm{NB} \left( \gamma_k^{(i-1)} \sum_{k2=1}^K \psi^{(i-1)}_{kk_1k_2}\pi_{k_2k}^{(i-1)}, \frac{-\mathrm{ln}\left(1-q_k^{(i)} \right)}{c_k^{(i)}-\mathrm{ln}\left( 1-q_k^{(i)}\right)}\right). \nonumber
\end{equation}
Then using Lemma 1, we sample
\begin{equation}
\label{g_kk_gam}
    \left(g_{k_1k}^{(i)}\mid -\right) \sim \mathrm{CRT} \left( h_{k_1k}^{(i)}, \gamma_k^{(i-1)} \sum_{k2=1}^K \psi^{(i-1)}_{kk_1k_2}\pi_{k_2k}^{(i-1)}\right),
\end{equation}
and obtain
\begin{equation}
\label{g_ikk}
    g_{k_1k}^{(i)} \sim \mathrm{Pois} \left(\gamma_k^{(i-1)} \sum_{k2=1}^K \psi^{(i-1)}_{kk_1k_2}\pi_{k_2k}^{(i-1)} \mathrm{ln} \left(1 - \mathrm{ln}\left( 1-q_k^{(i)}\right) \big/ {c_k^{(i)}} \right) \right).\nonumber
\end{equation}
If we define $g_{k_1k}^{(i)}=g_{k_1\cdot k}^{(i)}=\sum_{k2=1}^K g_{k_1k_2k}^{(i)}$, and augment
\begin{equation}
\label{g_kkk_gam}
    \left( g_{k_11k}^{(i)}, \cdots, g_{k_1Kk}^{(i)}\right) \sim \mathrm{Mult} \left(g_{k_1k}^{(i)}, \left( \psi^{(i-1)}_{kk_1k_2}\pi_{k_2k}^{(i-1)} \right)_{k_2=1}^K \right).
\end{equation}
By Lemma 3, we have
\begin{equation}
    g_{k_1k_2k}^{(i)} \sim \mathrm{Pois} \left( \gamma^{(i-1)} \psi^{(i-1)}_{kk_1k_2}\pi_{k_2k}^{(i-1)} \mathrm{ln} \left(1 - \mathrm{ln}\left( 1-q_k^{(i)}\right) \big/ {c_k^{(i)}} \right)\right). \nonumber
\end{equation}
Using Lemma 3 and $\sum_{k_1}^K \psi_{kk_1k_2}^{(i-1)}=1$, we have,
\begin{equation}
\label{g_mult_gam}
    \left( g_{\cdot 1k}^{(i)},\cdots, g_{\cdot Kk}^{(i)} \right) \sim \mathrm{Mult} \left( g_{\cdot k}^{(i)}, \left( \pi_{k_1k}^{(i-1)} \right)_{k_1=1}^K \right),
\end{equation}
\begin{equation}
    \left( g_{1k_2k}^{(i)}, \cdots, g_{Kk_2k}^{(i)} \right) \sim \mathrm{Mult} \left( g_{\cdot k_2k}^{(i)}, \left( \psi_{kk_1k_2}^{(i-1)} \right)_{k1=1}^{K} \right). \nonumber
\end{equation}
Thus by Dirichlet-multinomial conjugacy, for $i=I,\cdots,2$, we can obtain
\begin{align}
\label{psi_gam}
    \left( \left( \psi_{k1k_2}^{(i-1)}, \cdots, \psi_{kKk_2}^{(i-1)} \right) \mid -\right) & \sim  \mathrm{Dir} \left( \epsilon_0 + g_{1k_2k}^{(i)}, \cdots, \epsilon_0 + g_{Kk_2k}^{(i)} \right), \\
    \left( \boldsymbol{\pi}_k^{(i-1)} \mid - \right) & \sim \mathrm{Dir} \left( \alpha_{1k}^{(i-1)}+l_{1k}^{(i-1)}+g_{\cdot 1k}^{(i)},\cdots, \alpha_{Kk}^{(i-1)}+l_{Kk}^{(i-1)}+g_{\cdot Kk}^{(i)} \right). \label{pi_gam}
\end{align}
For sampling $\gamma_k^{(i-1)}$, note that by Eq.(\ref{g_ikk}) and $\sum_{k_1}^K \psi_{kk_1k_2}^{(i-1)}=1$, we have
\begin{equation}
    g_{\cdot k}^{(i)} = \sum_{k_1=1}^K g_{k_1k}^{(i)} \; \mathrm{and} \; g_{\cdot k}^{(i)} \sim \mathrm{Pois} \left( \gamma_k^{(i-1)} \mathrm{ln} \left(1 - \mathrm{ln}\left( 1-q_k^{(i)}\right) \big/ {c_k^{(i)}} \right) \right).
\end{equation}
Thus via Poisson-gamma conjugacy, we obtain
\begin{equation}
\label{gam_gam}
    \left(\gamma_k^{(i-1)}\mid-\right) \sim \mathrm{Gam} \left( \epsilon_0 + g_{\cdot k}^{(i)},  \epsilon_0 + \mathrm{ln} \left(1 - \mathrm{ln}\left( 1-q_k^{(i)}\right) \right) \right).
\end{equation}
By gamma-gamma conjugacy, we have
\begin{equation}
\label{c_ik}
    \left( c_k^{(i)}\mid -\right) \sim \mathrm{Gam} \left(\epsilon_0 + \gamma_k^{(i-1)}, \epsilon_0 + \sum_{k_1=1}^K \alpha_{k_1k}^{(i)}\right).
\end{equation}

\noindent\textbf{Inference for Dirichlet-Randomized-Gamma-Dirichlet Markov chains.} For Dirichlet-Randomized-Gamma-Dirichlet Markov chains,
\begin{equation}
\label{alpha_pr_gam}
    \alpha_{k_1k}^{(i)} \sim \mathrm{RG1} \left( \epsilon^\alpha, \gamma^{(i-1)} \sum_{k2=1}^K \psi^{(i-1)}_{kk_1k_2}\pi_{k_2k}^{(i-1)}, c_k^{(i)}\right), \nonumber
\end{equation}
which can be equivalently represent as
\begin{align}
    \alpha_{k_1k}^{(i)} \sim \mathrm{Gam} \left( g_{k_1k}^{(i)} + \epsilon^\alpha, c_k^{(i)} \right), \; \mathrm{and} \; g_{k_1k}^{(i)} = \mathrm{Pois} \left( \gamma^{(i-1)} \sum_{k2=1}^K \psi^{(i-1)}_{kk_1k_2}\pi_{k_2k}^{(i-1)} \right). \nonumber
\end{align}
By Eq.(\ref{l_kk_mult}), $\left( l_{1k}^{(i)}, \cdots, l_{Kk}^{(i)}\right)$ is multinomial distributed. If we marginalize $\left( \pi_{1k}^{(i)}, \cdots, \pi_{Kk}^{(i)} \right)$, $\left( l_{1k}^{(i)}, \cdots, l_{Kk}^{(i)}\right)$ will be Dirichlet-multinomial distributed. Thus by Lemma 2, for $i=I$, we first sample the auxiliary variables as
\begin{align}
    \left( q_k^{(I)} \mid -\right)  \sim \mathrm{Beta} \left( l_{\cdot k}^{(I)}, \alpha_{\cdot k}^{(I)}\right) \; \mathrm{and} \; \left(h_{k_1k}^{(I)} \mid - \right)  \sim \mathrm{CRT} \left( l_{k_1k}^{(I)}, \alpha_{k_1k}^{(I)}\right). \label{q_h_I_pr_gam}
\end{align}
Similarly, by Eq.(\ref{g_mult_pr_gam}), $\left( g_{\cdot 1k}^{(i)},\cdots, g_{\cdot Kk}^{(i)} \right)$ is also Dirichlet-multinomial distributed. Thus for $i=I-1,\cdots,2$, we sample the auxiliary variables as
\begin{align}
    \left( q_k^{(i)} \mid -\right)  \sim \mathrm{Beta} \left( l_{\cdot k}^{(i)} + g_{\cdot k}^{(i+1)}, \alpha_{\cdot k}^{(i)}\right) \; \mathrm{and} \; \left(h_{k_1k}^{(i)} \mid - \right) \sim \mathrm{CRT} \left( l_{k_1k}^{(i)}+ + g_{\cdot k_1 k}^{(i+1)}, \alpha_{k_1k}^{(i)}\right). \label{q_h_i_pr_gam}
\end{align}
Via Lemma 2, conditioning on $q_k^{(i)}$, we have
\begin{equation}
    \left( l_{k_1k}^{(i)} + g_{\cdot k_1 k}^{(i+1)}\right) \sim \mathrm{NB} \left( \alpha_{k_1k}^{(i)}, q_k^{(i)} \right). \nonumber
\end{equation}
Then via Lemma 1, we obtain
\begin{equation}
\label{H_iK_pr_gam}
    h_{k_1k}^{(i)} \sim \mathrm{Pois} \left( -\alpha_{k_1k}^{(i)} \mathrm{ln} \left( 1 - q_k^{(i)} \right) \right). \nonumber
\end{equation}
Via Poisson-gamma conjugacy, we first sample
\begin{equation}
    \left( \alpha_{k_1k}^{(i)} \mid - \right) \sim \mathrm{Gam} \left( g_{k_1k}^{(i)}+\epsilon^{\alpha}+h_{k_1k}^{(i)}, c_k^{(i)}-\mathrm{ln}\left( 1-q_k^{(i)}\right)\right).
\end{equation}
If $\epsilon^{\alpha} \textgreater 0$, we can sample the posterior of $g_{k_1k}^{(i)}$ via
\begin{equation}
\label{g_kk_bessel}
    \left( g_{k_1k}^{(i)} \mid - \right) \sim \mathrm{Bessel} \left( \epsilon^\alpha-1, 2 \sqrt{\alpha_{k_1k}^{(i)}c_k^{(i)}\gamma_k^{(i-1)}\sum_{k2=1}^K \psi^{(i-1)}_{kk_1k_2}\pi_{k_2k}^{(i-1)}}\right),
\end{equation}
where $\mathrm{Bessel} \left( \cdot \right)$ denotes Bessel distribution. If $\epsilon^\alpha = 0$, we sample $g_{k_1k}^{(i)}$ via
\begin{equation}
\label{g_kk_sch}
    \left( g_{k_1k}^{(i)} \mid - \right) \sim 
    \left\{ 
    \begin{array}{cc}
        \mathrm{Pois} \left( \frac{c_k^{(i)}\gamma_k^{(i-1)}\sum_{k2=1}^K \psi^{(i-1)}_{kk_1k_2}\pi_{k_2k}^{(i-1)}}{c_k^{(i)}-\mathrm{ln}\left(1 - q_k^{(i)} \right)} \right) & \mathrm{if} \; h_{k_1k}^{(i)}=0\\
        \mathrm{SCH}\left( h_{k_1k}^{(i)}, \frac{c_k^{(i)}\gamma_k^{(i-1)}\sum_{k2=1}^K \psi^{(i-1)}_{kk_1k_2}\pi_{k_2k}^{(i-1)}}{c_k^{(i)}-\mathrm{ln}\left(1 - q_k^{(i)} \right)}\right) & \mathrm{otherwise},
    \end{array} \right.
\end{equation}
where $\mathrm{SCH} \left( \cdot \right)$ denotes the shifted confluent hypergeometric distribution~\cite{schein2019poisson}.

Defining $g_{k_1k}^{(i)}=g_{k_1\cdot k}^{(i)}=\sum_{k2=1}^K g_{k_1k_2k}^{(i)}$, we first augment
\begin{equation}
\label{g_kkk_pr_gam}
    \left( g_{k_11k}^{(i)}, \cdots, g_{k_1Kk}^{(i)}\right) \sim \mathrm{Mult} \left(g_{k_1k}^{(i)}, \left( \psi^{(i-1)}_{kk_1k_2}\pi_{k_2k}^{(i-1)} \right)_{k_2=1}^K \right).
\end{equation}
By Lemma 3, we have
\begin{equation}
    g_{k_1k_2k}^{(i)} \sim \mathrm{Pois} \left(\gamma^{(i-1)} \psi^{(i-1)}_{kk_1k_2}\pi_{k_2k}^{(i-1)}\right), \nonumber
\end{equation}
and because $\sum_{k_1}^K \psi_{kk_1k_2}^{(i-1)}=1$, we have
\begin{align}
    \left( g_{\cdot 1k}^{(i)},\cdots, g_{\cdot Kk}^{(i)} \right) & \sim \mathrm{Mult} \left( g_{\cdot k}^{(i)}, \left( \pi_{k_1k}^{(i-1)} \right)_{k_1=1}^K \right), \, \mathrm{and} \label{g_mult_pr_gam}\\
    \left( g_{1k_2k}^{(i)}, \cdots, g_{Kk_2k}^{(i)} \right) & \sim \mathrm{Mult} \left( g_{\cdot k_2k}^{(i)}, \left( \psi_{kk_1k_2}^{(i-1)} \right)_{k1=1}^{K} \right).\nonumber
\end{align}
Thus by Dirichlet-multinomial conjugacy, for $i=I,\cdots,2$, we have
\begin{equation}
\label{psi_pr_gam}
    \left( \left( \psi_{k1k_2}^{(i-1)}, \cdots, \psi_{kKk_2}^{(i-1)} \right) \mid -\right) \sim  \mathrm{Dir} \left( \epsilon_0 + g_{1k_2k}^{(i)}, \cdots, \epsilon_0 + g_{Kk_2k}^{(i)} \right)
\end{equation}
\begin{equation}
\label{pi_pr_gam}
    \left( \boldsymbol{\pi}_k^{(i-1)} \mid - \right) \sim \mathrm{Dir} \left( \alpha_{1k}^{(i-1)}+l_{1k}^{(i-1)}+g_{\cdot 1k}^{(i)},\cdots, \alpha_{Kk}^{(i-1)}+l_{Kk}^{(i-1)}+g_{\cdot Kk}^{(i)} \right)
\end{equation}
Via Poisson-gamma conjugacy, we obtain
\begin{equation}
\label{gam_pr_gam}
    \left(\gamma_k^{(i-1)}\mid-\right) \sim \mathrm{Gam} \left( \epsilon_0 + g_{\cdot k}^{(i)}, \epsilon_0 + 1 \right).
\end{equation}
By gamma-gamma conjugacy, we have
\begin{equation}
\label{c_pr_gam}
    \left( c_k^{(i)}\mid -\right) \sim \mathrm{Gam} \left(\epsilon_0 + \gamma_k^{(i-1)}, \epsilon_0 + \sum_{k_1=1}^K \alpha_{k_1k}^{(i)}\right).
\end{equation}
Specifically, for $i=1$, we have
%\begin{equation}
%\label{pi_1}
%    \left( \boldsymbol{\pi}_k^{(1)} \mid - \right) \sim \mathrm{Dir} \left( \nu_1 \nu_k + l_{1k}^{(1)} + h_{1k}^{(2)}, \cdots, \xi \nu_k + l_{kk}^{(1)} + h_{kk}^{(2)}, \cdots,\nu_K \nu_k + l_{Kk}^{(1)} + h_{Kk}^{(2)} \right).
%\end{equation}
$\alpha_{k_1k}^{(1)}=\nu_{k_1}\nu_k$, if $k_1 \ne k$. And $\alpha_{k_1k}^{(1)}=\xi \nu_k$, if $k_1=k$.

\noindent \textbf{Sampling $\nu_k$ and $\xi$ :} As we sample $\bm{\Pi}^{(i)}$, by the definition of Dirichlet-multinomial distribution, we obtain
%\begin{equation}
%    \big( l_{1k}^{(1)}, \cdots, l_{Kk}^{(1)}\big) \sim \mathrm{DirMult} \left( \nu_1 \nu_K, \cdots, \xi \nu_k, \cdots, \nu_K \nu_k \right), \nonumber
%\end{equation}
\begin{equation}
    \big( l_{1k}^{(1)}+g_{\cdot 1k}^{(2)}, \cdots, l_{Kk}^{(1)}+g_{\cdot Kk}^{(2)}\big) \sim \mathrm{DirMult} \left( \nu_1 \nu_K, \cdots, \xi \nu_k, \cdots, \nu_K \nu_k \right), \nonumber
\end{equation}
where $l_{k_1k}^{(1)} = \sum_{t=1}^M l_{k_1k}^{(t)}$. In particular, with a little abuse of notation here, for Dir-Dir construction, we take $g_{\cdot k_1k}^{(2)}=h_{k_1k}^{(2)}$.
%\begin{equation}
%    \big( l_{1k}^{(1)}+g_{\cdot 1k}^{(2)}, \cdots, l_{Kk}^{(1)}+g_{\cdot Kk}^{(2)}\big) \sim \mathrm{DirMult} \left( \nu_1 \nu_K, \cdots, \xi \nu_k, \cdots, \nu_K \nu_k \right), \nonumber
%\end{equation}
We first sample 
\begin{equation}
\label{h_1}
    \left(h_{k_1k}^{(1)} \mid - \right) \sim \left\{
    \begin{array}{cc}
         \mathrm{CRT} \left( l_{k_1k}^{(1)}+g_{\cdot k_1k}^{(2)}, \nu_{k_1} \nu_k \right) &  k_1 \neq k\\
         \mathrm{CRT} \left( l_{k_1k}^{(1)}+g_{\cdot k_1k}^{(2)}, \xi \nu_k \right) & k_1 = k.
    \end{array} \right.
\end{equation}
Then we sample
\begin{equation}
\label{q_1}
    q_k^{(1)} \sim \mathrm{Beta} \left( l_{\cdot k}^{(1)}+g_{\cdot k}^{(2)}, \nu_k \left( \sum_{k_1 \neq k} \nu_{k1} + \xi \right) \right).
\end{equation}
We further introduce
\begin{align}
    n_k = & h_{kk}^{(1)} + \sum_{k_1 \neq k} h_{k_1k}^{(1)} + \sum_{k_2 \neq k} h_{kk_2}^{(1)} + l_{k\cdot}^{(1)}, \, \mathrm{and} \nonumber \\
    \rho_k = & \tau_0 \zeta^{(1)} -\mathrm{ln} \left( 1 - q_k^{(1)} \right) \left( \xi + \sum_{k_1 \neq k} \nu_{k_1} \right) - \sum_{k_2 \neq k} \mathrm{ln} \left( 1 - q_{k_2}^{(1)} \right) \nu_{k_2}. \nonumber
\end{align}
Via Poisson-gamma conjugacy, we have
\begin{align}
    \left( \xi \mid - \right) & \sim \mathrm{Gam} \left( \frac{\gamma_0}{K} + \sum_k h_{kk}^{(1)}, \beta - \sum_{k} \nu_k \mathrm{ln} \left( 1 - q_k^{(1)} \right)\right), \label{xi}\\
    \left( \nu_k \mid - \right) & \sim \mathrm{Gam} \left( \frac{\gamma_0}{K} + n_k, \beta + \rho_k \right). \label{nu}
\end{align}
\\
\noindent \textbf{Sampling $\delta^{(t)}$ and $\beta$ :} Via Poisson-gamma conjugacy
\begin{equation}
\label{delta_t}
    \left( \delta^{(t)} \mid - \right) \sim \mathrm{Gam} \left( \epsilon_0 + \sum_{v=1}^V y_v^{(t)}, \epsilon_0 + \sum_{k=1}^K \theta_k^{(t)} \right).
\end{equation}
And by gamma-gamma conjugacy, we obtain
\begin{equation}
\label{beta}
    \left( \beta \mid -\right) \sim \mathrm{Gam} \left( \epsilon_0 + \gamma_0, \epsilon_0 + \sum_{k=1}^K \nu_k \right).
\end{equation}
The full procedure of our Gibbs sampling algorithms are summarized in Algorithm~\ref{alg:mcmc_dir-dir}, Algorithm~\ref{alg:mcmc_dir-gam-dir} and Algorithm~\ref{alg:mcmc_pr-gam-dir}.
\begin{algorithm}[htbp]
   \caption{Gibbs sampling algorithm for NS-PGDS (Dir-Dir)}
   \label{alg:mcmc_dir-dir}
\begin{algorithmic}
 \STATE {\bfseries Input:} observed count sequence $\{\bm{y}^{(t)}\}_{t=1}^{\scriptstyle T}$, iterations $\mathcal{J}$.
   \STATE {\bfseries Initialize} the model's rank $K$, hyperparameters $\gamma_0, \epsilon_0, e_0, f_0$.
  %\REPEAT
  \FOR{$iter = 1$ {to} $\mathcal{J}$}
  \STATE {Sample $\{y_{vk}^{\scriptstyle(t)}\}_{v,k}$ via Eq.(\ref{y_vk}).}
  \STATE {Sample $\{\bm{\phi_k}\}_{k}$ via Eq.(\ref{phi_k}).}
  \STATE {Sample $\{\delta^{(t)}\}_{t}$ via Eq.(\ref{delta_t}). Update $\zeta^{(t)}$ as}\\
     \quad $\zeta^{(T+1)} = 0$,\quad $\zeta^{(t)} = \mathrm{ln} \left( 1 + \frac{\delta^{(t)}}{\tau_0} + \zeta^{(t+1)} \right), \; t=T,\cdots,1$.\;
     
   Set $l_{\cdot k}^{(T+1)} = 0$. \FOR{$t = T$ to $2$}
   \STATE {Sample $\{l_{k\cdot}^{(t)}\}_{k}$ and $\{l_{kk_2}^{(t)}\}_{k,k_2}$ via Eq.(\ref{l_k}) and Eq.(\ref{l_kk}) respectively.}
   \ENDFOR
   \FOR{$t = 1$ {to} $T$}
   \STATE {Sample $\{\theta_{k}^{(t)}\}_{k}$ via Eq.(\ref{theta_1}) and Eq.(\ref{theta_t}).}
   \ENDFOR
   \FOR{$i = 1$ {to} $I$}
   \STATE {Sample $\{q_k^{(i)}\}_{k}$ and $\{h_{k_1k}^{(i)}\}_{k_1,k}$ via Eq.(\ref{q_h_i}), Eq.(\ref{h_1}) and Eq.(\ref{q_1}).}
   \STATE {Sample $\{\bm{\pi}_k^{(i)}\}_{k}$ via Eq.(\ref{pi_I}) and Eq.(\ref{pi_i}).}
   \STATE {Sample $\eta$ via Eq.(\ref{eta}).}
   \ENDFOR
   \STATE {Sample $\xi$, $\{\nu_k\}_{k}$, $\beta$ via Eq.(\ref{xi}), Eq.(\ref{nu}) and Eq.(\ref{beta}) respectively.}
 \ENDFOR
 \STATE {\bfseries Output posterior means:} $\{\theta_{k}^{\scriptstyle (1:T)}\}_{k}$, $\{\bm{\phi}_k\}_{k}$, $\{\bm{\pi}_k^{(i)}\}_{k}$, $ \delta^{(1:T)}$, $\xi$, $\{\nu_k\}_{k}$, $\beta$.
\end{algorithmic}
\vskip -0.05in
\end{algorithm}

\begin{algorithm}[htbp]
   \caption{Gibbs sampling algorithm for NS-PGDS (Dir-Gam-Dir)}
   \label{alg:mcmc_dir-gam-dir}
\begin{algorithmic}
 \STATE {\bfseries Input:} observed count sequence $\{\bm{y}^{(t)}\}_{t=1}^{\scriptstyle T}$, iterations $\mathcal{J}$.
   \STATE {\bfseries Initialize} the model's rank $K$, hyperparameters $\gamma_0, \epsilon_0, e_0, f_0$.
  %\REPEAT
  \FOR{$iter = 1$ {to} $\mathcal{J}$}
  \STATE {Sample $\{y_{vk}^{\scriptstyle(t)}\}_{v,k}$ via Eq.(\ref{y_vk}).}
  \STATE {Sample $\{\bm{\phi_k}\}_{k}$ via Eq.(\ref{phi_k}).}
  \STATE {Sample $\{\delta^{(t)}\}_{t}$ via Eq.(\ref{delta_t}). Update $\zeta^{(t)}$ as}\\
     \quad $\zeta^{(T+1)} = 0$,\quad $\zeta^{(t)} = \mathrm{ln} \left( 1 + \frac{\delta^{(t)}}{\tau_0} + \zeta^{(t+1)} \right), \; t=T,\cdots,1$.\;
     
   Set $l_{\cdot k}^{(T+1)} = 0$. \FOR{$t = T$ to $2$}
   \STATE {Sample $\{l_{k\cdot}^{(t)}\}_{k}$ and $\{l_{kk_2}^{(t)}\}_{k,k_2}$ via Eq.(\ref{l_k}) and Eq.(\ref{l_kk}) respectively.}
   \ENDFOR
   \FOR{$t = 1$ {to} $T$}
   \STATE {Sample $\{\theta_{k}^{(t)}\}_{k}$ via Eq.(\ref{theta_1}) and Eq.(\ref{theta_t}).}
   \ENDFOR
   \FOR{$i = 1$ {to} $I$}
   \STATE {Sample $\{\alpha_{k_1k}^{(i)}\}_{k_1,k}$ and $\{c_k^{(i)}\}_{k}$ via Eq.(\ref{alpha_gam})} and Eq.(\ref{c_ik}).
   \STATE {Sample $\{q_k^{(i)}\}_{k}$ and $\{h_{k_1k}^{(i)}\}_{k_1,k}$ via Eq.(\ref{q_h_I_gam}), Eq.(\ref{q_h_i_gam}), Eq.(\ref{h_1}) and Eq.(\ref{q_1}).}
   %\STATE {Sample $\{h_{k_1k}^{(i)}\}_{k_1,k}$ via Eq.(\ref{h_1}) and Eq.(\ref{h_i}) respectively.}
   \STATE {Sample $\{g_{k_1k}\}_{k_1, k}$ and $\{g_{k_1k_2k}\}_{k_1,k_2,k}$ via Eq.(\ref{g_kk_gam}) and Eq.(\ref{g_kkk_gam}) respectively.}
   \STATE {Sample $\{\psi_{kk_1k_2}\}_{k,k_1,k_2}$ via Eq.(\ref{psi_gam}).}
   \STATE {Sample $\{\gamma_k^{(i)} \}_k$ via Eq.(\ref{gam_gam}).}
   \STATE {Sample $\{\bm{\pi}_k^{(i)}\}_{k}$ via Eq.(\ref{pi_I}) and Eq.(\ref{pi_gam}).}
   \ENDFOR
   \STATE {Sample $\xi$, $\{\nu_k\}_{k}$, $\beta$ via Eq.(\ref{xi}), Eq.(\ref{nu}) and Eq.(\ref{beta}) respectively.}
 \ENDFOR
 \STATE {\bfseries Output posterior means:} $\{\theta_{k}^{\scriptstyle (1:T)}\}_{k}$, $\{\bm{\phi}_k\}_{k}$, $\{\bm{\pi}_k^{(i)}\}_{k}$, $ \delta^{(1:T)}$, $\xi$, $\{\nu_k\}_{k}$, $\beta$.
\end{algorithmic}
\vskip -0.05in
\end{algorithm}

\begin{algorithm}[t]
   \caption{Gibbs sampling algorithm for NS-PGDS (PR-Gam-Dir)}
   \label{alg:mcmc_pr-gam-dir}
\begin{algorithmic}
 \STATE {\bfseries Input:} observed count sequence $\{\bm{y}^{(t)}\}_{t=1}^{\scriptstyle T}$, iterations $\mathcal{J}$.
   \STATE {\bfseries Initialize} the model's rank $K$, hyperparameters $\gamma_0, \epsilon_0, e_0, f_0$.
  %\REPEAT
  \FOR{$iter = 1$ {to} $\mathcal{J}$}
  \STATE {Sample $\{y_{vk}^{\scriptstyle(t)}\}_{v,k}$ via Eq.(\ref{y_vk}).}
  \STATE {Sample $\{\bm{\phi_k}\}_{k}$ via Eq.(\ref{phi_k}).}
  \STATE {Sample $\{\delta^{(t)}\}_{t}$ via Eq.(\ref{delta_t}). Update $\zeta^{(t)}$ as}\\
     \quad $\zeta^{(T+1)} = 0$,\quad $\zeta^{(t)} = \mathrm{ln} \left( 1 + \frac{\delta^{(t)}}{\tau_0} + \zeta^{(t+1)} \right), \; t=T,\cdots,1$.\;
     
   Set $l_{\cdot k}^{(T+1)} = 0$. \FOR{$t = T$ to $2$}
   \STATE {Sample $\{l_{k\cdot}^{(t)}\}_{k}$ and $\{l_{kk_2}^{(t)}\}_{k,k_2}$ via Eq.(\ref{l_k}) and Eq.(\ref{l_kk}) respectively.}
   \ENDFOR
   \FOR{$t = 1$ {to} $T$}
   \STATE {Sample $\{\theta_{k}^{(t)}\}_{k}$ via Eq.(\ref{theta_1}) and Eq.(\ref{theta_t}).}
   \ENDFOR
   \FOR{$i = 1$ {to} $I$}
   \STATE {Sample $\{\alpha_{k_1k}^{(i)}\}_{k_1,k}$ and $\{c_k^{(i)}\}_{k}$ via Eq.(\ref{alpha_pr_gam})} and Eq.(\ref{c_pr_gam}).
   \STATE {Sample $\{q_k^{(i)}\}_{k}$ and $\{h_{k_1k}^{(i)}\}_{k_1,k}$ via Eq.(\ref{q_h_I_pr_gam}), Eq.(\ref{q_h_i_pr_gam}), Eq.(\ref{h_1}) and Eq.(\ref{q_1}).}
   %\STATE {Sample $\{h_{k_1k}^{(i)}\}_{k_1,k}$ via Eq.(\ref{h_1}) and Eq.(\ref{h_i}) respectively.}
   \STATE {Sample $\{g_{k_1k}\}_{k_1, k}$ via Eq.(\ref{g_kk_bessel}) and Eq.(\ref{g_kk_sch}).}
   \STATE {Sample $\{g_{k_1k_2k}\}_{k_1,k_2,k}$ via Eq.(\ref{g_kkk_pr_gam}).}
   \STATE {Sample $\{\gamma_k^{(i)} \}_k$ via Eq.(\ref{gam_pr_gam}).}
   \STATE {Sample $\{\psi_{kk_1k_2}\}_{k,k_1,k_2}$ via Eq.(\ref{psi_pr_gam}).}
   \STATE {Sample $\{\bm{\pi}_k^{(i)}\}_{k}$ via Eq.(\ref{pi_I}), and Eq.(\ref{pi_pr_gam}).}
   \ENDFOR
   \STATE {Sample $\xi$, $\{\nu_k\}_{k}$, $\beta$ via Eq.(\ref{xi}), Eq.(\ref{nu}) and Eq.(\ref{beta}) respectively.}
 \ENDFOR
 \STATE {\bfseries Output posterior means:} $\{\theta_{k}^{\scriptstyle (1:T)}\}_{k}$, $\{\bm{\phi}_k\}_{k}$, $\{\bm{\pi}_k^{(i)}\}_{k}$, $ \delta^{(1:T)}$, $\xi$, $\{\nu_k\}_{k}$, $\beta$.
\end{algorithmic}
\vskip -0.05in
\end{algorithm}
